# Supplementary material for: Confidence-based Out-of-Distribution Detection: A Comparative Study and Analysis
Source: arXiv:2107.02568 source file (2021-07-06)
Supplement: Supplementary file 1 [file appendix.tex]

\noindent\textbf{Ps\_1m\_Segm:} \comment{DELETE THIS. PUT IT AS PART OF THE NEXT SECTION: We investigate the performance of transductive learning via pseudo-labels, without the use of a confidence threshold. We train a model from scratch, optimizing the training object \comment{REFERENCE} over the labeled data of DB1 and pseudo-labels for DB2. The latter are the segmentations produced by a model supervised solely on DB1, from experiments \emph{Superv.DB1}. The predictions of the model on DB2 at the last iteration of training are evaluated against manual segmentations on DB2. We repeat the experiments 10 times with different seeds, each using as pseudo-labels the segmentations from one of the 10 experiments \emph{Superv.DB1} and report the average performance. This method corresponds to the commonly-used SSL method \cite{lee2013pseudo}, previously used in a variety of works for induction, but is here evaluated in a transductive setup. We find that on average across the 7 classes, the method does not improve the results. Intuitively, this can be explained by the fact that the method does not provide \emph{new} information about the relation between images and labels. Previous works that found it useful for inductive SSL have coupled it with a form of regularization of the segmentations, such as via the use of a CRF for refining the pseudo-labels \cite{bai2017semi}. However configuring such a shape-based regularizer is not straightforward nor reliable in segmentation tasks with multiple classes, which differ in shape and size of different shapes such as the one studied here. Hence we seek to induce extra information in more flexible manner. \comment{THESE COMMENTS SHOULD BE IN THE METHOD SECTION.}}

\noindent\textbf{Ps\_Ens\_Segm and Ps\_Ens\_C-$t$:} Quality of pseudo-labels relates to how the quality of initial predictions, and the information gain by applying a confidence threshold relates to how well calibrated is the model's confidence, as described in Sec.~\comment{(REF)}. To investigate this empirically, we construct an ensemble of the 10 fully-supervised models (Superv.DB1) and obtain the ensemble's class-posterior probability maps for DB2 by averaging the predicted posteriors by these 10 models. We then create pseudo-labels with the same steps as previously described for the Ps.1m.Segm and Ps.1m.C-$t$ experiments, but derived from the ensemble's output. We repeat the experiments based on pseudo-labels that match the ensemble's segmentation (Ps.Ens.Segm), as well as experiments with pseudo-labels constructed via $7$ values of confidence threshold $t$ (Ps.Ens.C-$t$). Each experiment is repeated with 10 different seeds and we report the average performance for each setting in Tab.~\ref{tab:dice_ps1m_01} and Fig.~\comment{(REF)}. Threshold-based pseudo-labeling improves over using the actual model segmentations as targets, as well as entropy minimization. Moreover, we find that the performance improvements offered by applying a confidence threshold at different values follow a similar trend as the information gain we calculated in Sec.~\comment{REFERENCE}, confirming our hypothesis. This is a useful insight, as it provides indication towards constructing more easy to calibrate transductive methods: One should strive for developing models with well-calibrated confidence, and then positive information gain can be obtained via thresholds in the areas even close to 0.5 (the more calibrated, the  closer).

\noindent\textbf{Ens(experiment):} 
The previous experiments offered insights about the importance of quality of prediction and confidence calibration and showed ensemble-based pseudo-labels offer benefits.
To be useful in practice, however, such a method must improve the ensemble itself. For each previous experiment \comment{CAREFUL, I MAY HAVE TO CHOOSE, BECAUSE SPACE}, we construct an ensemble by averaging the class-posteriors of the $10$ models trained with different seeds. Because of limited space, we present representative results in detail in Tab.~\ref{tab:dice_ps1m_01}, and plot the average performance across all classes in for all experiments Fig.~\comment{REF}. Ens(Superv.DB1) is the ensemble used for creating the pseudo-labels in the experiments \emph{Ps\_Ens\_XXX} above. We observe that ensembles of models trained with transductive learning outperform the baseline ensemble of fully-supervised models across all classes for a wide range of values of confidence thresholds $t$ between values $0.6-0.99$.

\begin{table}[t]
	\begin{center}
	%\centering
	%\small 
	%\setlength{\tabcolsep}{4pt}
	\begin{tabular}{@{}lcccccc|c@{}}
	    \toprule
		\textbf{Method} & \textbf{Core} & \textbf{Oed.} & \textbf{NoTBI} & \textbf{Probe} & \textbf{Pet.}  & \textbf{Intrav.} & \textbf{Avg.} \\
        \midrule % Or \hline, it does not break the vertical line
		Ps\_Ens\_0.7 (100\%unl.)        & $57.3$ & $46.4$ & $33.8$ & $50.7$ & $21.1$ & $50.1$  & $43.2$ \\
		Ps\_Ens\_0.7 (50\% unl.)        & $55.3$ & $46.4$ & $34.0$ & $48.9$ & $20.3$ & $54.6$  & $43.3$ \\
		%Ps\_Ens\_0.7 (50\% unl.)-Induct.& $50.5$ & $43.5$ & $32.7$ & $41.8$ & $19.9$ & $49.7$  & $39.7$ \\
		Ps\_Ens\_0.9 (100\%unl.)        & $57.1$ & $45.8$ & $34.6$ & $52.2$ & $22.1$ & $53.9$  & $44.3$ \\
		Ps\_Ens\_0.9 (50\% unl.)        & $56.4$ & $44.3$ & $33.2$ & $56.9$ & $23.5$ & $61.4$  & $45.9$ \\
		%Ps\_Ens\_0.9 (50\% unl.)-Induct.& $52.7$ & $42.1$ & $31.6$ & $50.6$ & $22.8$ & $57.1$  & $42.8$ \\
		\midrule
		Ens(Ps\_Ens\_0.7)                    & $61.9$ & $51.8$ & $35.2$ & $63.2$ & $23.9$ & $57.0$  & $48.8$ \\
		Ens(Ps\_Ens\_0.7)(50\% unl.)         & $63.0$ & $50.5$ & $34.1$ & $63.2$ & $26.1$ & $67.8$  & $50.8$ \\
		%Ens(Ps\_Ens\_0.7)(50\% unl.)-Induct. & $62.9$ & $47.5$ & $39.6$ & $56.1$ & $26.5$ & $60.1$  & $48.8$ \\
		Ens(Ps\_Ens\_0.9)                    & $61.4$ & $48.9$ & $39.6$ & $67.6$ & $30.2$ & $68.0$  & $52.6$ \\
		Ens(Ps\_Ens\_0.9)(50\% unl.)         & $63.0$ & $47.5$ & $39.8$ & $75.3$ & $32.9$ & $75.9$  & $55.6$ \\
		%Ens(Ps\_Ens\_0.9)(50\% unl.)-Induct. & $61.5$ & $48.2$ & $35.9$ & $68.5$ & $32.8$ & $69.0$  & $52.7$ \\
		\bottomrule
	\end{tabular}
	\caption{Transductive learning with $100\%$ and $50\%$ unlabelled data from DB2 used for training. Tranductive learning works well even with unlabelled data. \comment{(MERGE WITH TABLE 1 FOR SPACE?)}}
	%\caption{Transductive learning with $100\%$ and $50\%$ unlabelled data from DB2 used for training, and performance of inductive SSL. Tranductive learning works well even with less data, and better than inductive SSL.}
	\label{tab:less_data_transd_induct}
		\end{center}
\end{table}

\begin{table}[t]
	\begin{center}
	%\centering
	%\small 
	%\setlength{\tabcolsep}{4pt}
	\begin{tabular}{@{}lcccccc|c@{}}
	    \toprule
		\textbf{Method} & \textbf{Core} & \textbf{Oed.} & \textbf{Non-TBI} & \textbf{Probe} & \textbf{Petech.}  & \textbf{Intrav.} & \textbf{Average} \\
        \midrule % Or \hline, it does not break the vertical line
		Sup.DB1 (baseline)  & $32.1$ & $32.4$ & $20.8$ & $28.5$ & $15.6$ & $39.4$  & $28.1$ \\ 
		Sup.DB1.DB2 &$36.1$ &$42.0$ &$30.1$ & $49.8$ & $22.2$ & $55.0$  & $39.2$ \\ % 5-fold superv.
		\midrule
		Entr.Min.   & $51.8$ & $43.1$ & $26.8$ & $46.6$ & $17.6$ & $46.6$  & $38.8$ \\
		Ps.1m.Segm \cite{lee2013pseudo} & $43.4$ & $37.7$ & $21.5$ & $23.2$ & $15.6$ & $31.5$  & $28.8$ \\
		\midrule
		Ps.1m.C0.5  & $42.6$ & $39.3$ & $23.0$ & $25.9$ & $15.3$ & $30.8$  & $29.5$ \\
		Ps.1m.C0.6  & $47.8$ & $41.3$ & $23.4$ & $27.5$ & $16.3$ & $34.5$  & $31.8$ \\
		Ps.1m.C0.7  & $47.0$ & $42.1$ & $24.6$ & $28.1$ & $16.1$ & $34.0$  & $32.0$ \\
		Ps.1m.C0.8  & $52.8$ & $44.4$ & $24.7$ & $35.4$ & $18.1$ & $39.0$  & $35.7$ \\
		Ps.1m.C0.9  & $55.2$ & $44.4$ & $27.0$ & $38.6$ & $18.1$ & $45.4$  & $38.1$ \\
		Ps.1m.C0.95 & $56.1$ & $44.1$ & $28.8$ & $39.3$ & $18.8$ & $41.0$  & $38.0$ \\
		Ps.1m.C0.99 & $54.4$ & $43.6$ & $28.2$ & $43.4$ & $21.1$ & $48.4$  & $39.9$ \\
		\midrule % Or \hline, it does not break the vertical line
		Ps.Ens.Segm  & $51.4$ & $46.1$ & $31.9$ & $38.9$ & $17.9$ & $39.7$  & $37.7$ \\
		\midrule
		Ps.Ens.C0.5  & $52.2$ & $45.2$ & $30.3$ & $36.9$ & $17.4$ & $42.4$  & $37.4$ \\
		Ps.Ens.C0.6  & $55.1$ & $46.6$ & $33.0$ & $43.3$ & $18.7$ & $47.7$  & $40.7$ \\
		Ps.Ens.C0.7  & $57.3$ & $46.4$ & $33.8$ & $50.7$ & $21.1$ & $50.1$  & $43.2$ \\
		Ps.Ens.C0.8  & $58.5$ & $46.4$ & $34.2$ & $52.7$ & $22.2$ & $54.5$  & $44.8$ \\
		Ps.Ens.C0.9  & $57.1$ & $45.8$ & $34.6$ & $52.2$ & $22.1$ & $53.9$  & $44.3$ \\
		Ps.Ens.C0.95 & $57.4$ & $45.3$ & $32.3$ & $50.0$ & $24.5$ & $54.2$  & $44.0$ \\
		Ps.Ens.C0.99 & $53.5$ & $41.4$ & $27.8$ & $46.9$ & $20.3$ & $52.1$  & $40.3$ \\
		\bottomrule
	\end{tabular}
	\caption{Performance of \emph{single models}, measured via the \emph{average Dice-Sorensen Coefficient} (\%) \textbf{over all cases}. When there is no lesion of a class, DC is defined equal to 1 if prediction agrees there is no class, or 0 if there has been a false positive.} % Valid Dice.
	\label{tab:dice_ps1m_01}
		\end{center}
\end{table}

\begin{abstract}
    My abstract is commonly around 15-19 lines. My abstract is commonly around 15-19 lines. My abstract is commonly around 15-19 lines. My abstract is commonly around 15-19 lines. My abstract is commonly around 15-19 lines. My abstract is commonly around 15-19 lines. My abstract is commonly around 15-19 lines. My abstract is commonly around 15-19 lines. My abstract is commonly around 15-19 lines. My abstract is commonly around 15-19 lines. My abstract is commonly around 15-19 lines. My abstract is commonly around 15-19 lines. My abstract is commonly around 15-19 lines. My abstract is commonly around 15-19 lines. My abstract is commonly around 15-19 lines. My abstract is commonly around 15-19 lines. My abstract is commonly around 15-19 lines. My abstract is commonly around 15-19 lines. My abstract is commonly around 15-19 lines. My abstract is commonly around 15-19 lines. My abstract is commonly around 15-19 lines. 
\end{abstract}

\begin{abstract}
    Semi-supervised learning (SSL) aims to utilize unlabelled data during training to learn a model that makes better predictions. Previous works on SSL for medical image segmentation have focused on improving the model's generalization to new, unseen data. In many applications, however, our ultimate goal is to obtain predictions on a predefined unlabelled database, available at the time of model's development, and not generalization. Such an example are retrospective studies for extracting image-based phenotypes from existing databases. Therefore this study investigates SSL from a different perspective: We evaluate the quality of predictions made on the unlabelled data of interest when they are included during training and optimized over. For this, we revisit two existing SSL methods, self-supervision and entropy minimization. We explore how they benefit learning from an information theoretic perspective, which gives insights in how to improve the framework and untap its potential. Experiments on multi-center data for multi-class segmentation of traumatic brain injuries show that making predictions via transduction on the target data greatly improves those obtained by induction from supervised models. We believe the promising results of this study will inspire further research on the field of transduction, which is well-suited for various medical image analysis studies.
\end{abstract}
